# Supplementary material for: FASTer: Focal Token Acquiring-and-Scaling Transformer for Long-term 3D Object Detection
Source: arXiv:2503.01899 source file (2025-02-28)
Supplement: Supplementary file 1 [file X_suppl.tex]

\clearpage
\setcounter{page}{1}
\maketitlesupplementary
\appendix
\begin{table*}[]
\belowrulesep=0pt
 \aboverulesep=0pt
  \centering
  \small
  \begin{tabular}{c|c|cc|cc|cc|cc}
  \hline
    \toprule
\centering   
   \multirow{2}{*}{\centering Method} & \multirow{2}{*}{Stage} & \multicolumn{2}{c}{ALL (mAPH)} & \multicolumn{2}{|c}{VEH (AP/APH)}  & \multicolumn{2}{|c}{PED (AP/APH)} & \multicolumn{2}{|c}{CYC (AP/APH)}  \\
\cline{3-10} & & L1 & L2 &  L1 &  L2 & L1  & L2 & L1 & L2  \\
 
    \midrule
% \centering  SST-3f\cite{sst} & 3 &- &- &78.66/78.21& 69.98/69.57 &83.81/80.14& 75.94/72.37 &-& -\\
\centering  CenterPoint-4f\cite{centerpoint} &1 & 74.30 &  68.71 & 76.68/76.13& 69.09/68.58& 78.58/75.51 & 71.25/68.37 & 72.20/71.28 & 70.10/69.20 \\

\centering  +FASTer    & 2    & 81.49 & 75.92 & 83.21/82.77  & 75.81/75.37  & 85.94/83.35  & 79.14/76.61 & 79.09/78.37 & 76.80/76.10\\
\midrule

\centering DSVT-4f \cite{dsvt} & 1 &   81.3 & 75.6 & 81.8 / 81.4 &74.1 / 73.6 & 85.6 / 82.8 & 78.6 / 75.9 & 80.4 / 79.6 & 78.1 / 77.3\\
\centering   +FASTer    &2      & 82.99 & 77.26 & 84.08/83.71  & 77.03/77.60  & 86.88/84.42  & 80.44/78.16 & 81.69/80.85 & 79.93/76.02\\

% \midrule
\centering Scatterformer-4f\cite{scatterformer} & 1  & 81.5 & 76.5  & 82.7 / 81.9 & 75.0 / 74.5 & 86.5 / 83.7 & 80.2 / 77.5 &79.8 / 79.0 &78.5 / 77.4 \\
\centering  +FASTer    &2      & 83.55 & 78.39 & 84.81/84.38  & 77.76/77.34  & 87.65/85.32  & 81.19/78.88 & 81.85/80.97 & 80.03/78.97\\

% \midrule
% FASTer(Ours)  & 2      & \textbf{81.62} & \textbf{76.06} & 83.53/83.02  & 76.14/75.41  & \textbf{85.99}/\textbf{83.39}  & 79.17/\textbf{76.62} & \textbf{79.18/78.45} & \textbf{76.86/76.17}\\

    \bottomrule
\hline
  \end{tabular}
  \caption{Extra comparative experiments on the validation set of Waymo Open Dataset. }
  \label{tab:extra_result}
\end{table*}    

\begin{figure*}
    \centering
    \includegraphics[width=1.0\linewidth]{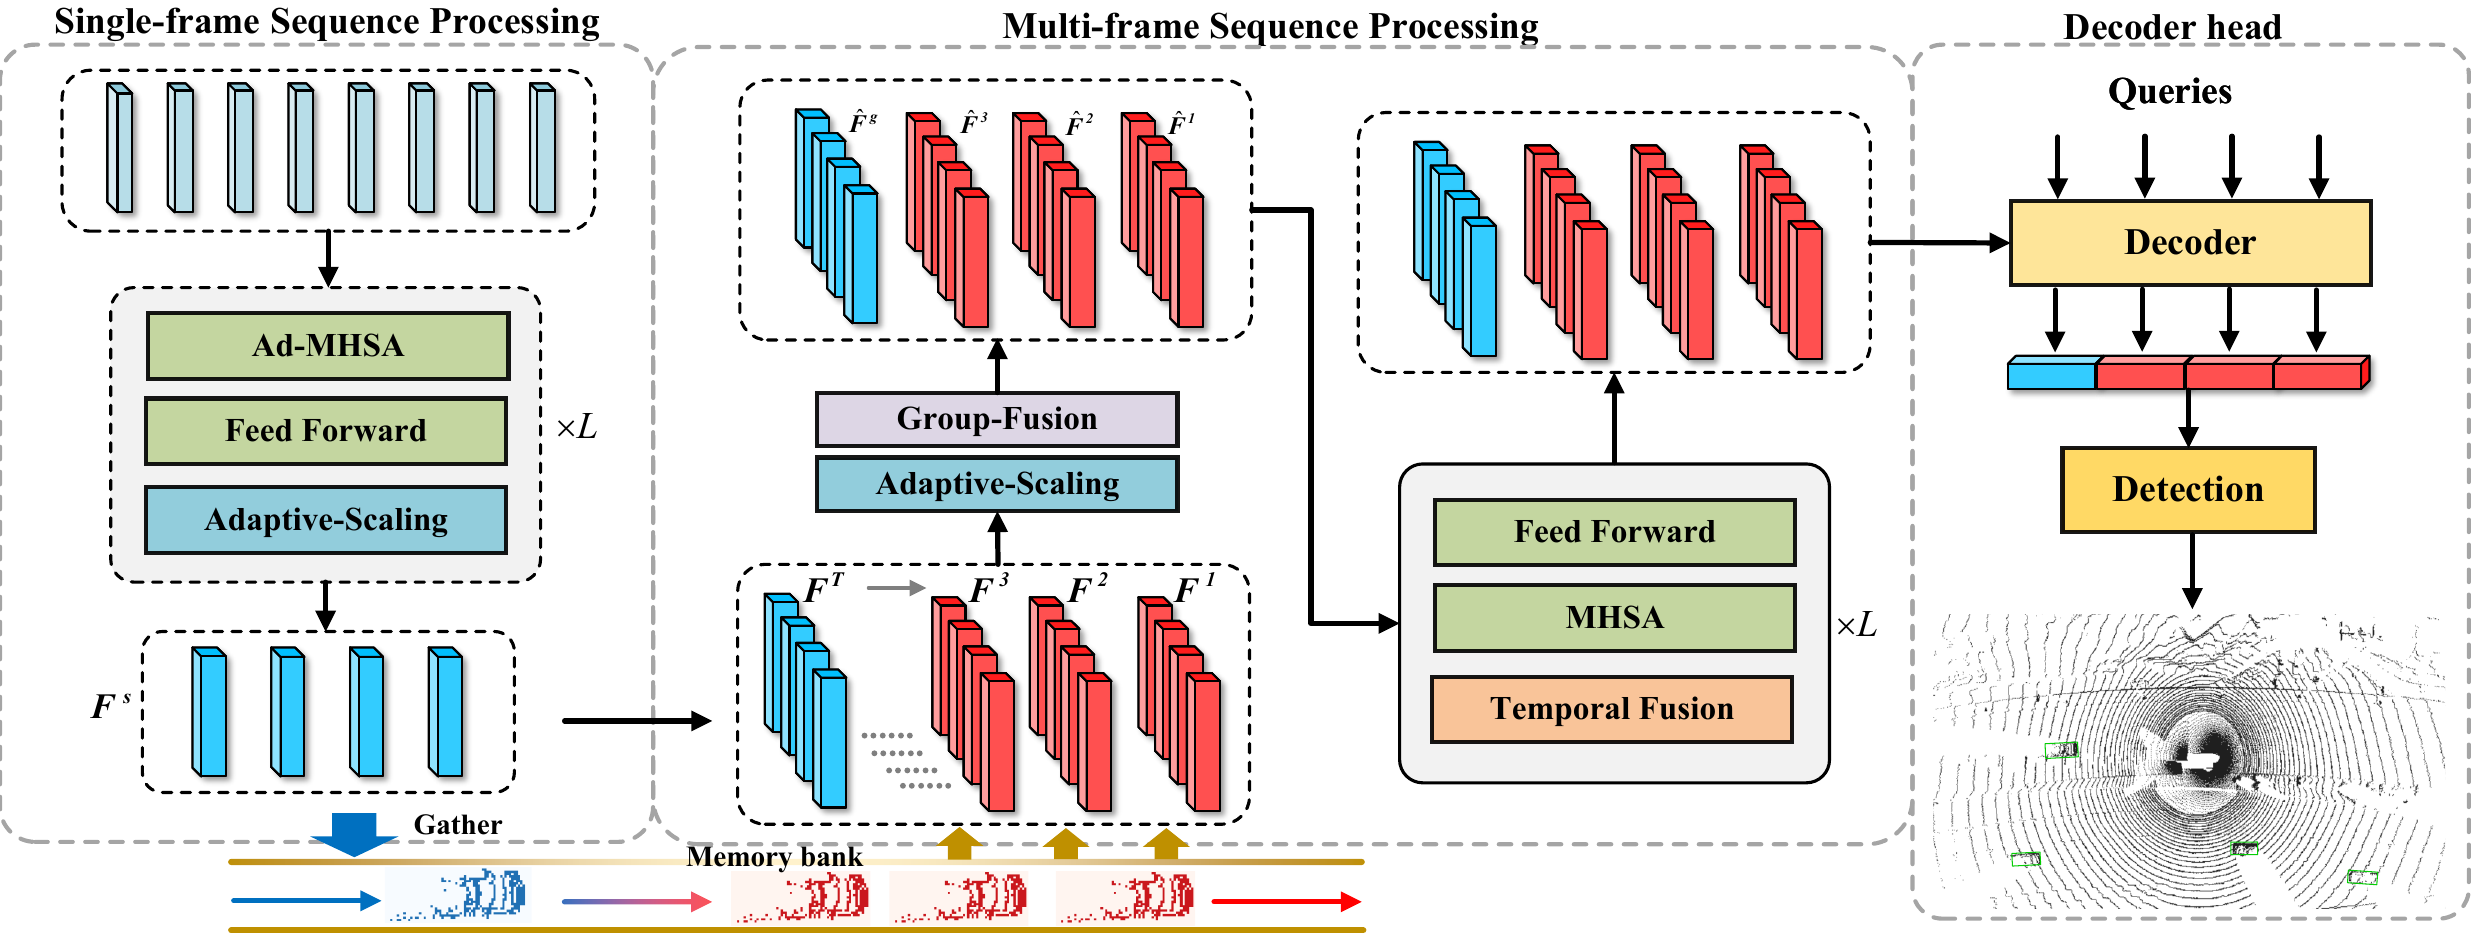}
    \caption{The details of the result-level concatenation network in our ablation experiments. The Single-frame Sequence Processing is identical to that of FASTer. In the Multi-frame Sequence Processing, multiple compressed sequences are fed into the multi-layer temporal-geometric fusion module. Each sequence is then decoded using a Transformer decoder and thehe outputs from all groups are concatenated for detection. Notably, we sequentially employ BiFA in \cite{msf} and Cross Attention inspired by \cite{mppnet} for temporal fusion.}
    \label{fig:faster+bifa}
\end{figure*}

\section{Extra results}
\setlength{\tabcolsep}{5.5pt}

To ensure a fair comparison with existing two-stage methods, we deliberately employ a suboptimal Sparse-CNN as the backbone in our approach, though the backbone can be substituted with any ones. To further validate the effectiveness of our proposal-based method, we present experimental results in which a powerful transformer is used as the backbone alongside our FASTer (16-frame) as the ROI-Head. Data augmentation techniques, including ground-truth sampling, random flipping, rotation, scaling, and translation, are applied consistently. All other hyper-parameters follow the official settings without modification. We also employ a uniform center-based dense head across experiments. 

As presented in \cref{tab:extra_result}, the results reveal that, although substituting the backbone significantly enhances proposal quality, FASTer still demonstrates substantial improvements in bounding box refinement, pushing performance closer to the upper limits achievable in Lidar-based detection tasks. Our experiments reveal that the recall rate of proposals is critical to the final optimization outcome.

% \section{Rationale}
% \label{sec:rationale}
% % 
% Having the supplementary compiled together with the main paper means that:
% % 
% \begin{itemize}
% \item The supplementary can back-reference sections of the main paper, for example, we can refer to \cref{sec:intro};
% \item The main paper can forward reference sub-sections within the supplementary explicitly (e.g. referring to a particular experiment); 
% \item When submitted to arXiv, the supplementary will already included at the end of the paper.
% \end{itemize}
% % 
% To split the supplementary pages from the main paper, you can use \href{https://support.apple.com/en-ca/guide/preview/prvw11793/mac#:~:text=Delete%20a%20page%20from%20a,or%20choose%20Edit%20%3E%20Delete).}{Preview (on macOS)}, \href{https://www.adobe.com/acrobat/how-to/delete-pages-from-pdf.html#:~:text=Choose%20%E2%80%9CTools%E2%80%9D%20%3E%20%E2%80%9COrganize,or%20pages%20from%20the%20file.}{Adobe Acrobat} (on all OSs), as well as \href{https://superuser.com/questions/517986/is-it-possible-to-delete-some-pages-of-a-pdf-document}{command line tools}.

\section{Some Details}
\paragraph{Details of result-level concatenation variants.}
In this section, we provide the details of the result-level concatenation network, in our ablation experiments. As show in \cref{fig:faster+bifa}, the Single-frame Sequence Processing is identical to that of FASTer. In the Multi-frame Sequence Processing module, after the initial adaptive scaling and Group Fusion, multiple compressed sequences are fed into the multi-layer temporal-geometric fusion module. Each sequence is then decoded using a standard Transformer decoder and their outputs from all groups are concatenated for detection. Notably, we sequentially employ BiFA in \cite{msf} and Cross Attention inspired by \cite{mppnet} for temporal fusion. Experiments demonstrate that the absence of Adaptive Scaling mechanism significantly increases inference latency and adversely affects detection performance. We argue that the isolation of geometric fusion and temporal fusion impedes the flow of global information, resulting in abrupt changes in feature dimensions during result-level concatenation, which restricts the model's learning capacity.

\paragraph{Details of staged training and Extra Point Augmentation.}
Informative points are acquired through learning and cannot be obtained in advance. During the first three epochs of training, points from the history frame are sampled from the full point cloud. After three epochs, we use the existing model to infer the training set and generate informative points for further training. Following the fifth epoch, this process is repeated to update informative points. However, this significantly reduces the diversity of training set and makes the model more sensitive to the RPN. 

We select proposals with fewer points (28 in our experiments) from two preceding and two following frames, transform them to the current time, sample points from the remaining set, and storing them with the informative points. We refer to this operation as Extra Points Augmentation (EPA), which we believe mitigates FASTer's reliance on the RPN, and enhances the model's generalization on the validation set, as confirmed in our ablation studies. During inference, EPA is discarded, and only informative points from the SSP are retained.

\paragraph{Details of various token compression methods.}
We experimented with various token compression methods. 

For supervised token selection, a simple prediction head is added to the tokens to predict their scores, with direct supervision from the ground truth. Following \cite{pointrcnn}, a transition threshold $\eta$ is used to ensure smooth training. Specifically, we define point $p$ as lying within the box obtained by scaling the length, width, and height of Ground truth Box $B$ by a factor of $a$, the point-box supervision value $\hat{y}$ can be obtained as follows:
\begin{equation}
\hat{y} = \left\{
\begin{array}{ll}
1 & \text{if  } a<1-\eta \\
0 & \text{if  } a>1+\eta \\
\frac{1+\eta-a}{2\eta}&  \text{else}\\
\end{array}
\right.
\end{equation}
where $\eta$, in our implementation, is set to 0.2.

For attention masking implementation, inspired by \cite{dynamicvit}, we obtain the binary score for each token via Gumbel-Softmax\cite{gumbelsoftmax} technique, while ensuring the differentiability of training. Additionally, a masking operation is applied to the attention map to enable gradient updates. During the inference stage, the attention masking operation is omitted, and tokens are selected based on their scores.

\section{Visualization}
\begin{figure*}
    \centering
    \includegraphics[width=1.0\linewidth]{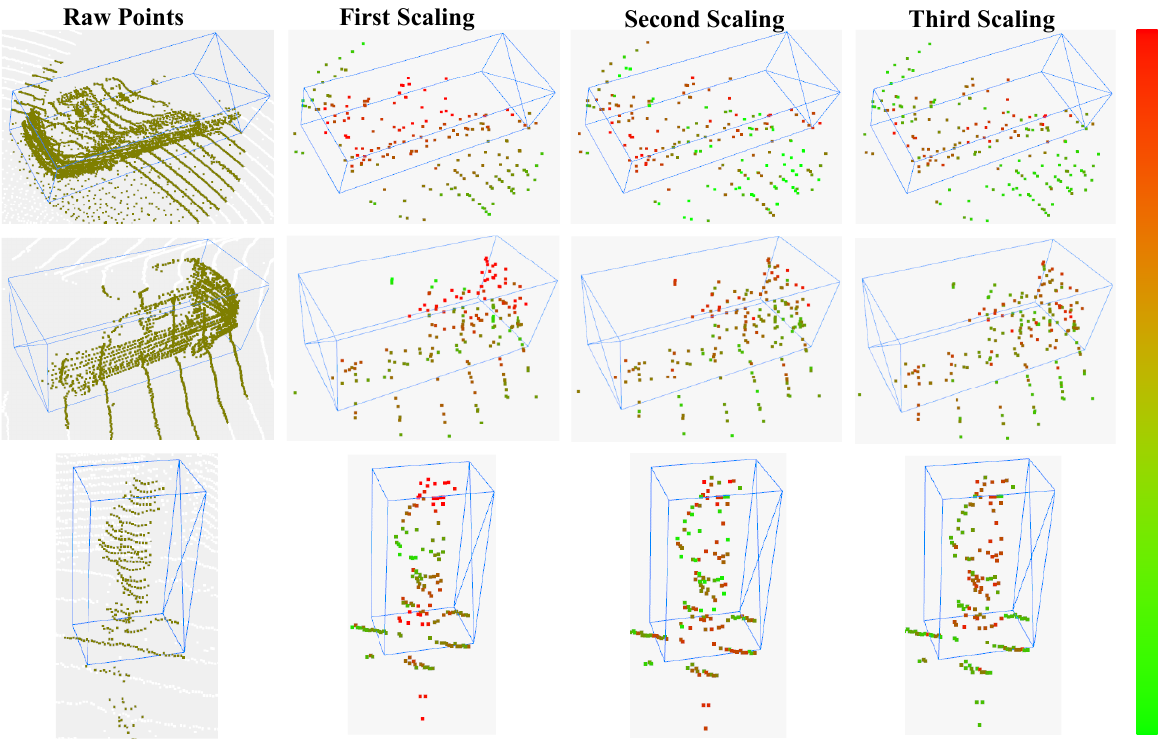}
    \caption{Token scores derived from several instances following different layers of adaptive scaling.}
    \label{fig:attention}
\end{figure*}

As illustrated in \cref{fig:attention}, we visualize the token scores of selected instances after each dynamic scaling operation. It is observed that the scores of points within the bounding box are significantly higher than those outside, which aligns with our general understanding. Interestingly, the score distribution in the initial layer is relatively concentrated and continuous, indicating that the model primarily focuses on local features. As the dynamic scaling progresses through multiple layers, the overall token score distribution becomes increasingly scattered and chaotic. This suggests that the model is gradually shifting its perspective from local details to a more global understanding of the instances.

\section{Extra experiments}
In this section, we give some other ablation experiments. The mAPH on L1 and L2 are reported in default.
\subsection{Effects of grouping strategies}
We design experiments to investigate the impact of different grouping strategies. As shown in \cref{tab:group}, we observed that, modifying the equidistant grouping to a single-stride grouping results in a significant decrease in detection scores. This finding indicates that our hierarchical grouping and fusion model is far from a mere aggregation of multi-frame point clouds. Instead, its rational and structured fusion strategy enhances the model's ability to extract long-term temporal features effectively.
\begin{table}[]
\belowrulesep=0pt
 \aboverulesep=-1.5pt
    \centering
    \begin{tabularx}{0.48\textwidth}{c| c c c } 
    \toprule
  % \hspace{0pt} $\hat{F}^1$  &  $\hat{F}^2$ &  $\hat{F}^3$ &  $\hat{F}^4$       \\
  %   \midrule
\rule{0pt}{2.5ex}  & Strategy 1 & Strategy 2& Strategy 3 \\  
\midrule
  Group1 &$\{1,5,9,13\}$&$\{1,2,3,4\}$&$\{1,2,3,4\}$\\

  Group2 & $\{2,6,10,14\}$&$\{5,6,7,8\}$&$\{1,3,5,7\}$\\

  Group3 & $\{3,7,11,15\}$&$\{9,10,11,12\}$&$\{1,4,7,10\}$\\
  Group4 & $\{4,8,12,16\}$&$\{13,14,15,16\}$&$\{1,5,9,13\}$\\
\midrule
mAPH   &81.49/75.92  & 80.92/75.37 & 81.01/75.44 \\ 
     
    \bottomrule
    \end{tabularx}
    \caption{Comparison of different grouping strategies. Each cell contains the index of the corresponding sequence within the complete temporal sequences of its respective group.}
    \label{tab:group}
\end{table}
\subsection{Effects of Scaling Ratio}
In the main body of our paper, for clarity, we assume that each adaptive scaling operation reduces a sequence to half of its original length, though this reduction ratio can be adjusted, enhancing the flexibility of FASTer. Specifically, let $\beta_1$ and $\beta_2$ denote the reduction ratios for Ad-MHSA in SSP and MSP respectively. By varying these ratios while maintaining a constant $K$, we present the comparative experimental results in \cref{tab:scaling ratio}. We observe that larger scaling ratios generally enhance performance by preserving more information, but excessive values can lead to redundant tokens. Our analysis indicates that the model is more sensitive to $\beta_2$ than $\beta_1$, as multi-frame sequences inherently encapsulate richer information. This suggests that frame count or point cloud density is a critical factor in determining the model’s performance limit.
\setlength{\tabcolsep}{4pt}

\subsection{Robustness Analysis}

\setlength{\tabcolsep}{4pt}
\begin{table}[]
\belowrulesep=0pt
 \aboverulesep=-0.9pt
    \centering
    \begin{tabularx}{0.48\textwidth}{c| c c c c} 
    \toprule

\diagbox{$\beta_1$}{$\beta_2$} & 0.6 & 0.5 & 0.4& 0.3\\
\midrule
  0.6 & 81.7 / 76.0 & 81.3 / 75.6  & 80.2 / 74.2 & 78.7 / 74.5 \\
  0.5 & 81.7 / 75.9 & 81.2 / 75.6 &  80.2 / 74.2 &  78.8 / 74.6 \\
  0.4 & 81.2 / 75.4 & 80.6 / 75.1 & 79.8 / 74.3 &  78.2 / 74.0\\
  0.3 & 80.6 / 74.7 & 79.9 / 74.5 & 79.1 / 73.7 & 77.5 / 73.2   \\
     
    \bottomrule
    \end{tabularx}
    \caption{Comparison of scaling ratios, $\beta_1$ for SSP, and $\beta_2$ for MSP.}
    \label{tab:scaling ratio}
\end{table}

\begin{table}[]
\belowrulesep=0pt
 \aboverulesep=-0.9pt
 \fontsize{9.3}{11}\selectfont
    \centering
    \begin{tabularx}{0.48\textwidth}{c| c c |c c} 
    \toprule
\rule{0pt}{2.5ex} \multirow{2}{*}{{\centering \makecell{Drop\\Rate}}} & \multicolumn{2}{c|}{Point Drop} & \multicolumn{2}{c}{Box Drop}\\
& FASTer &MSF  & FASTer &PTT \\
\midrule
  0 & 81.49/75.92 & 80.20/74.62  & 81.49/75.92 & 80.20/74.60  \\
  0.1 & 81.15/75.56 & 79.51/73.40 &  81.43/75.84 &  80.03/74.42 \\
  0.2 & 80.80/75.19 & 78.67/72.73 & 81.30/75.72 &  79.82/74.14\\
  0.3 & 80.30/74.67 & 77.58/71.54 & 81.15/75.58 & 79.58/73.89   \\
\bottomrule
    \end{tabularx}
    \caption{Comparison of the model's robustness when points or boxes are randomly dropped with a specified probability.}
    \label{tab:robustness}
\end{table}
To assess the robustness of FASTer under partial data loss, we randomly discard a subset of points or boxes from the historical frames during the inference phase, without additional training. The results are presented in \cref{tab:robustness}. 

Compared to boxes, FASTer exhibits a relatively higher sensitivity to points, while the impact of dropping boxes is minimal. This demonstrates that, within the context of region-guided temporal fusion, points play a more significant role and have a greater influence on the model performance than boxes. We hypothesize that points provide richer semantic information, whereas boxes mainly contribute limited geometric information. 

In comparison with other methods, MSF\cite{msf}, which relies solely on historical boxes, shows greater sensitivity to points, while PTT, which relies solely on historical boxes, exhibits stronger sensitivity to boxes than FASTer. These validate that FASTer maintains robust performance even in the presence of sensor malfunctions and data loss.
